# Supplementary material for: Is Support Set Diversity Necessary for Meta-Learning?
Source: arXiv:2011.14048 source file (2021-10-07)
Supplement: Supplementary file 1 [file appendix.tex]

\section*{Appendix}

\section{Over-parameterization is helpful?}

In our experiments we currently observe that \fixml matches or improves over \ml performance for a variety of base-learners but only for over-parameterized networks like Resnet-12. The performance on shallower networks like conv-64 is poorer than traditional \ml. \red{We are currently investigating some possible explanations for the played by over-parameterized architectures.}

\paragraph{Bias of \fixml.} \fixml minimizes a biased estimate of the inner task generalization error where as \ml minimizes an unbiased estimate of this. For an algorithm $\calA:\calZ^m \rightarrow \calH$ which maps $m$ training samples to a hypothesis, the generalization error on task on $\tau$ for the estimate $A(S), \, S \in \calZ^m$ is given by $ \E_{S,z|\tau} l(\calA(S), z)$. The expectation of the \ml objective for a task is: $\E_{(S,Q)|\tau} l(A(S), Q) = \E_{S|\tau} \calR_\tau(\calA(S))$.
Here $S$ is the R.V. denoting the support for the task $\tau$ and as we can see $l(A(S), Q)$ which is minimized by \ml for a set of sampled $(S, Q)$ pairs from a task is an unbiased estimate of the generalization error on task $\tau$.  

On the other hand, \fixml minimizes an unbiased estimate of the biased risk $\calR_\tau(\calA(S_{p,0}^{\tau}))$.
One hypothesis is that the bias faced by \fixml: $|\calR_\tau(\calA(S_{p,0}^{\tau})) - \E_S \calR_\tau(\calA(S))|$ when minimizing a biased version of the inner-task generalization gap, is large for shallower backbones as opposed to deep architectures. 

Both \fixml and \ml learn parameters for the same inner-task algorithm $\calA \in \{\calA\}$ but with two different dataset constructions: $\calD_{ml} = \{(S^i_k, Q^i_k)\}$ 
and $\calD_{fml} = \{(S_{p,0}^i, Q^i_k)\}$ where $i$ denotes the task and $k$ denotes the pair within the $i^{th}$ task. 
Let the meta-algorithm be denoted by $\Psi:\tau^n \rightarrow \{\calA\}$ such that \fixml returns
$\Psi(\calD_{fml})$ and \ml returns $\Psi(\calD_{ml})$. Intuitively, we can refer to the bias incurred by \fixml as the difference in the \ml objective's loss given by the \fixml solution
$\hat{\E}_{S,Q,\tau \sim \calD_{ml}} l(\Psi(\calD_{fml})(S),Q)$ and the \ml objective's loss given by the \ml solution $\hat{\E}_{S,Q,\tau \sim \calD_{ml}} l(\Psi(\calD_{ml})(S),Q)$ (Figure~\ref{fig:3}(c)). \red{We are currently investigating some possible directions to analyze (i) in which cases is the bias incurred by \fixml lower? (ii) What is the reason for \fixml to overcome this bias and still perform better?} \blue{We are looking at some directions from (i) model-free generalization analysis mainly done for initialization based methods in convex/linear settings and algorithm-dependent stability analysis (which is a bit unclear for meta-learning, but we give some notion of this as follows).}  
The generalization error for \fixml solution $\calA(\calD_{fml})$ can be broadly broken down into:

\begin{align}
&\abs{\hat{\E}_\tau \hat{\calR}_\tau(\calA(\calD_{fml})(S_{p,0}^\tau)) - \E_\tau \E_{S|\tau} \calR_\tau(\calA(\calD_{fml})(S))} \nonumber \\
&\leq \underbrace{\abs{\hat{\E}_\tau \hat{\calR}_\tau(\calA(\calD_{fml})(S_{p,0}^\tau)) - \hat{\E}_\tau \hat{E}_{S|\tau} \hat{\calR}_\tau(\calA(\calD_{fml})(S))}}_{\textrm{gap verified from trajectory plots}} \nonumber \\
&+ \abs{\hat{\E}_\tau \hat{E}_{S|\tau} \hat{\calR}_\tau(\calA(\calD_{fml})(S)) - \E_\tau \E_{S|\tau} \calR_\tau(\calA(\calD_{fml})(S))}
\label{eq:genn-gap}
\end{align}

The first term is a result of within task bias and the second term can be bounded using the stability of a meta-learner.

Question 1: For deep networks, can we show that \textbf{within-task-bias} for \fixml can be bounded above by a small value for over-parameterized networks (first term in Eq~\ref{eq:genn-gap})?

% \forall {\tau,S_{p,0},z} |l(\calA(\calD_{fml})(S_{p,0}^{\tau})) - \E_S \calR_\tau(\calA(\calD_{fml})(S))| \leq \Tilde{\gamma}

% The above term is loosely realized by the optimization trajectory plots. 

Question 2: Is the outer \textbf{outer-stability} for the \fixml solution better than \ml, which can explain \fixml achieving a lower value for the second term in Eq~\ref{eq:genn-gap} (compared to $ |\hat{\E}_\tau \hat{E}_{S|\tau} \hat{\calR}_\tau(\calA(\calD_{ml})(S)) - \E_\tau \E_{S|\tau} \calR_\tau(\calA(\calD_{ml})(S))|$)?

\textbf{Why:} The second term in the bound above measures the generalization gap of a solution on the empirical \ml objective and the true \ml objective on the task distribution. This can be bounded by $\epsilon(\Tilde{\gamma}, \gamma)$ where  $\Tilde{\gamma}$ is the stability of the inner-task algorithm and $\gamma$ is the stability of the outer algorithm. For both \fixml and \ml solutions the former is going to be same, since we are sampling a random support $S$ here. But the meta-algorithm's stability may be different given that the effective constructed datasets $\calD_{ml}$ and $\calD_{fml}$ are different.

% \begin{align}
%     & \sup_{D_{fml},S} \abs{\E_\tau \brck{ \calR_\tau(\calA(\calD_{fml})(S)) -  \E_{S|\tau} \calR_\tau(\calA(\calD_{fml}^{\backslash i})(S))}} \\
%     & \qquad \leq  \sup_{D_{ml},S}    \abs{\E_\tau\brck{ \E_{S|\tau}\calR_\tau(\calA(\calD_{ml})(S)) - \E_{S|\tau} \calR_\tau(\calA(\calD_{ml}^{\backslash i})(S))}} 
% \end{align}

\begin{figure*}[ht]
    \begin{minipage}[b]{0.45\textwidth}
    \centering
    \includegraphics[width=\linewidth]{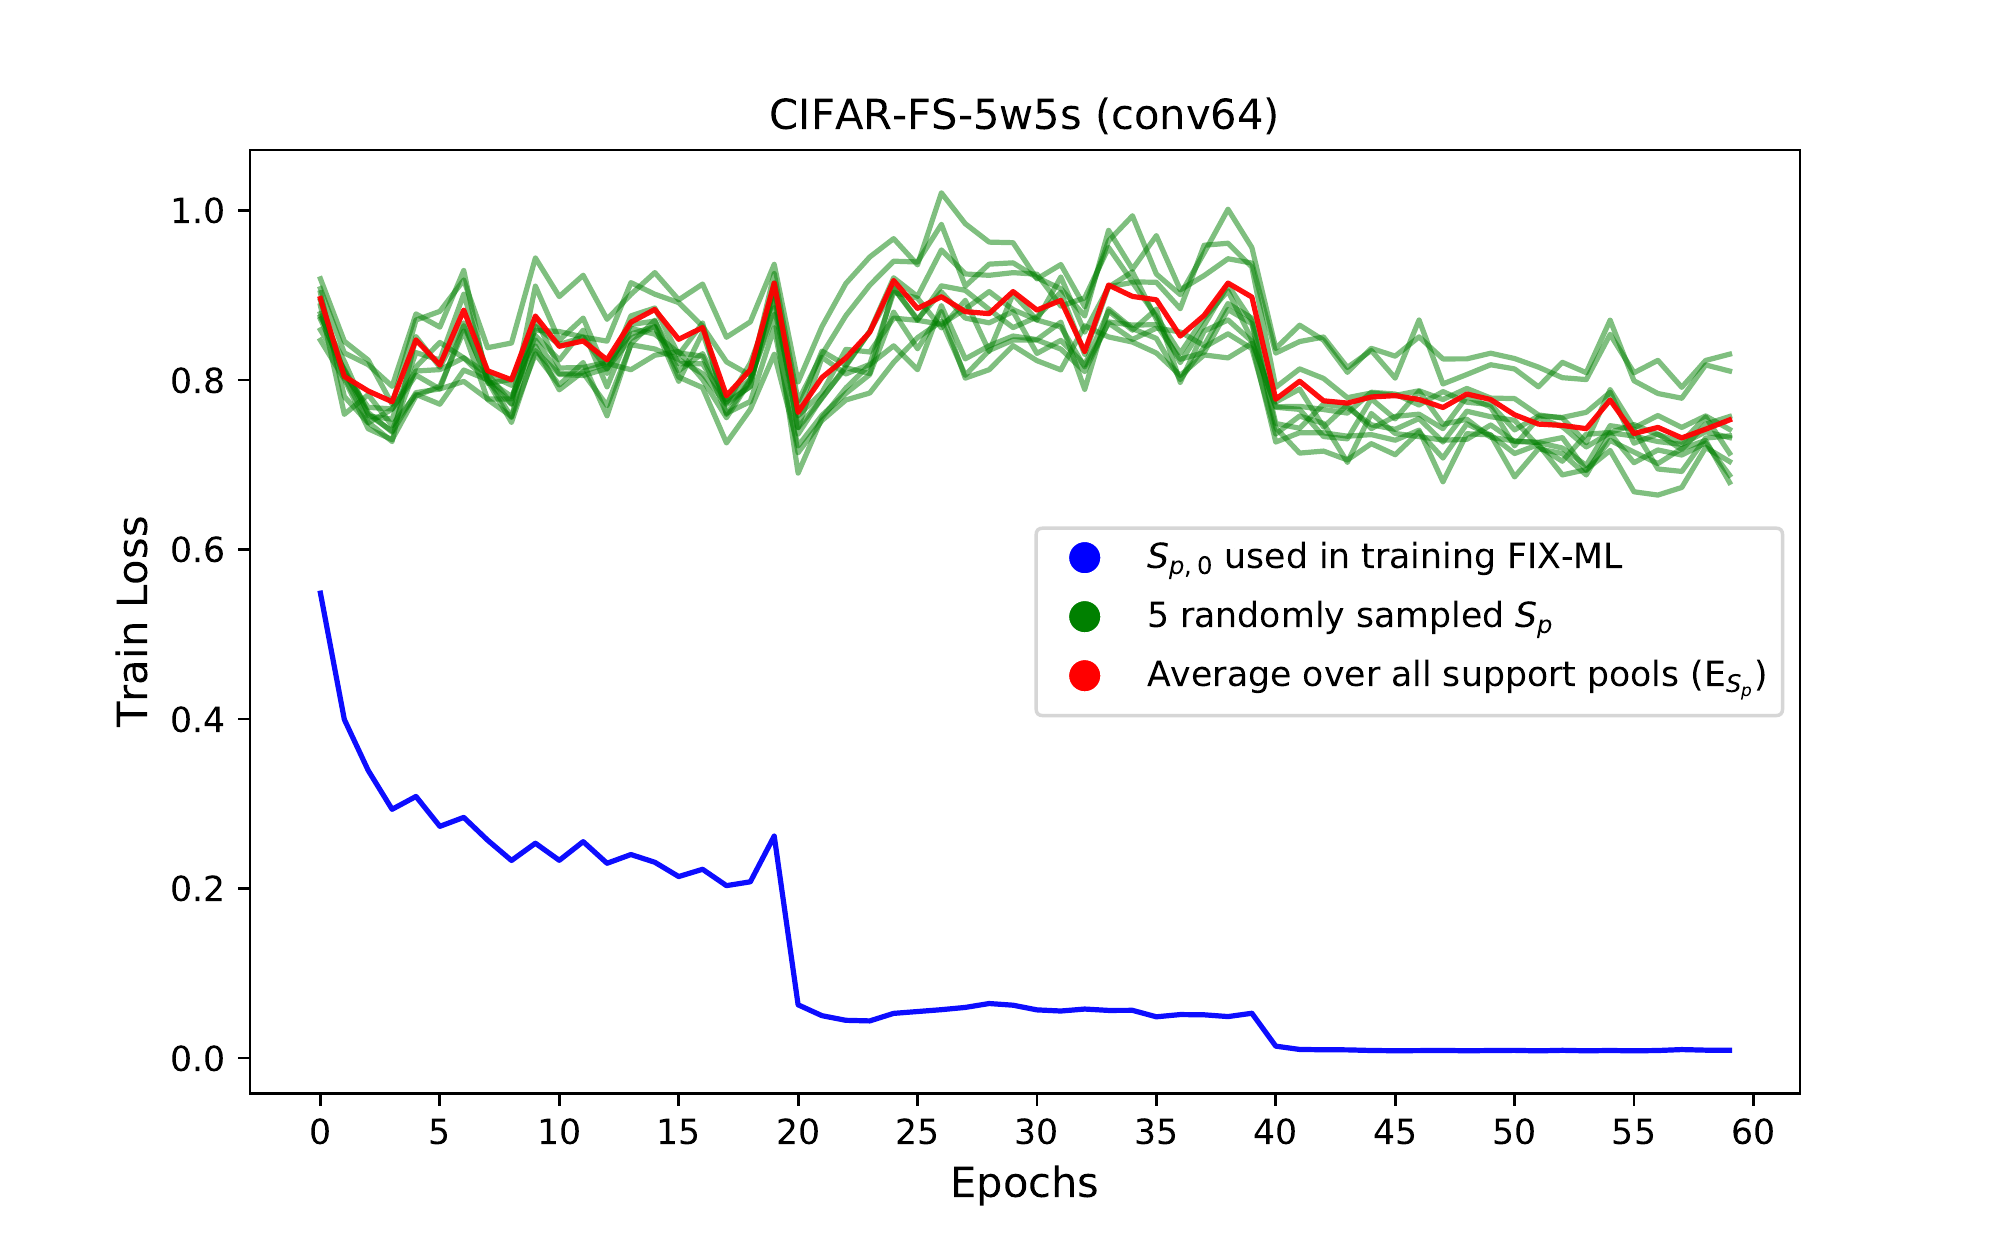}
    \captionsetup{labelformat=empty}
    % \caption*{(train)}
    \end{minipage}\hfill
    \begin{minipage}[b]{0.45\textwidth}
    \centering
    \includegraphics[width=0.82\linewidth]{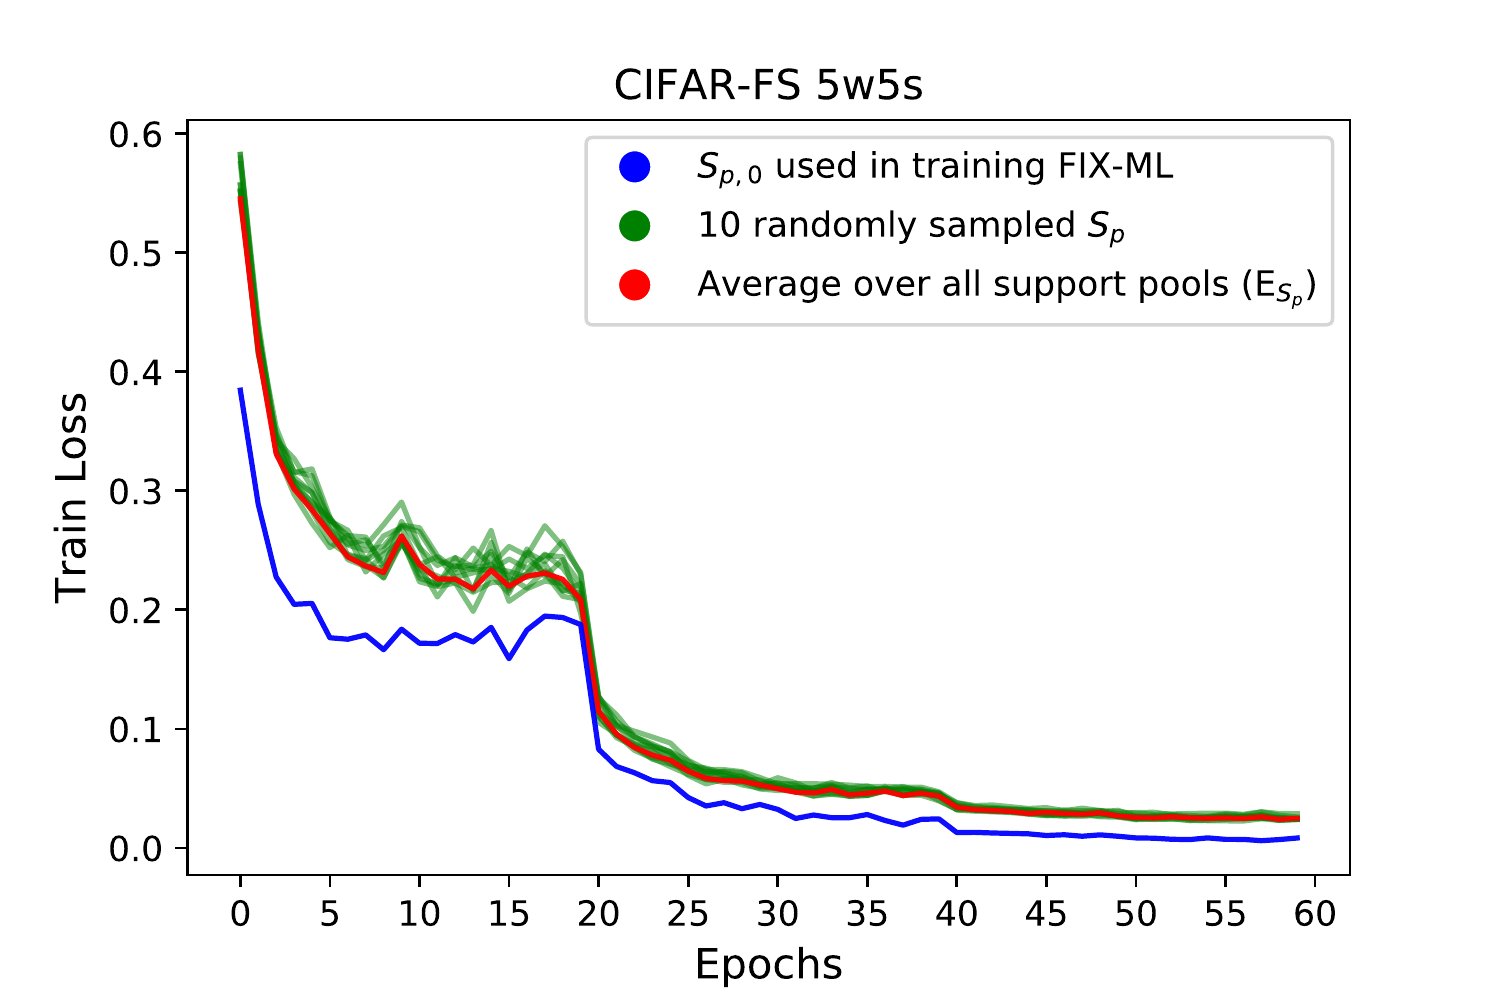}
    \captionsetup{labelformat=empty}
    % \caption*{(val)}
    \end{minipage}\hfill
    \caption{Comparison of trajectory plots for \fixml (evaluated on the fixed support and the \ml objective) for conv-64 (left) and Resnet (right). The gap between the blue and red curves is large for shallower networks, significantly increasing the within-task-bias (first term in Eq~\ref{eq:genn-gap}).}
    \label{fig:trajectory-compare}
\end{figure*}

% $|\calR(\calA(S_{p,0}^{C});\tau) - \calR(\calA(S);\tau)|$ where $S_{p,0}^{C}$ is the fixed support for the task. \fixml minimizes an unbiased estimator of this biased risk $\calR(\calA(S_{p,0}^{C});\tau)$. 

\section{Initialization Based Meta-learners}

\begin{table}[!th]
    \centering
    \begin{tabular}{c|c|c|c|c}
       \textbf{D/Alg} & \textbf{Arch.} & \textbf{Task Config} & \textbf{\ml} &\textbf{\fixml}   \\ \hline
        \cif/MAML  & Conv48   & 5w5s15q  &  $62.87 \pm 1.05\%$    & $60.64 \pm 1.13\%$   \\
        \cif/FOMAML & Conv48   & 5w5s15q  &   $ 61.21 \pm 1.20\%$   &  $58.01\pm1.07\%$ 
        % \cif/FOMAML  & Resnet-12   & 5w5s15q  & $\pm$   &   $\pm$ \\
        % \cif/Reptile & Resnet-12    & 5w5s15q  &    &    \\ \bottomrule
    \end{tabular}
    \vspace{1em}
    \caption{Comparing \ml and \fixml on MAML and its first-order approximations on Conv64 and Resnet}
    \label{tab:init-based}
\end{table}

\textbf{Comparison on \cif with Resnet-12: }\\
\ml meta-lr: 0.005 inner-loop: 5steps, $\alpha=0.01$ (79.59 performance)

\ml meta-lr: 0.02 inner-loop: 5steps, $\alpha=0.01$ (79.89, 80.19 performance)

(Variant-1) \fixml (no. of examples per class in support pool $5$) meta-lr: 0.005 inner-loop: 5steps, $\alpha=0.01$ (77.85 performance) 

(Variant-2) \fixml (no. of examples per class in support pool $5$) meta-lr: 0.02 inner-loop: 5steps, $\alpha=0.01$ (79.67 performance) 

(Variant-3) \fixml (no. of examples per class in support pool $60$) meta-lr: 0.005 inner-loop: 5steps, $\alpha=0.01$ (79.82 performance) 

\red{Two phenomenons that we observe:}

1. Before we drop learning rate at Epoch 35, we observe the double descent phenomena, where the test loss increases after a few epochs and then drops once we drop learning rate at epoch 35. This is observed for both ml and fixml. This is possibly one reason for why better optimization is not necessarily leading to better generalization \textbf{which has been the case in all the over-parameterized (Resnet based) models that we hve trained in the past.}

2. In some cases, we observe that test loss is not tracking test acc. This is not the case when we compare \fixml and \ml models with the same set of hyper-params, so it doesn't necessarily hinder our current conclusion that \fixml is closely matching (but slightly worse) than \ml for first-order MAML (with Resnet).

\begin{itemize}
    \item The performance gap drops for larger architectures.
    \item The behavior of \fixml's optimization is slightly different from last-layer methods in the sense that it is slower to converge w.r.t the \fixml objective. We observed the opposite for last-layer. This is possibly due to the first-order approximations that are made.
    \item check $0.02$ outer loop learning rate (do fixml still converge slower than ml in this hyperparameter?) \am{added graph for this (third row on next page), TL;DR it is still slower}
\end{itemize}

\red{We see that \fixml matches \ml performance but there is certainly room for further improvement, since convergence rate of \fixml is slow (more on the graphs on the next page).  One possible explanation can be that fix-ml doesn't play well with the first-order approximation in MAML:}

W/o the approx. the expected value of the meta-gradient w.r.t $\theta$: 
\begin{align}
   \E_{C}\E_{(S,Q)|C} \brck{\frac{\partial \phi}{\partial \theta} \nabla_{\phi} L(\phi; Q)}
\end{align}

Let's say $\phi(\theta, S) = \theta - \alpha \nabla_\theta L(\theta; S)$ and $\phi(\theta) = \theta - \alpha \nabla_\theta \E_S L(\theta; S)$, then the meta-gradient is: \os{Writing $\phi$ as a function of $S$ is important here. This might make the factorization over $S, Q$ impossible.}
\am{I do agree. I was looking into that just now and one way around that can be $\phi = \theta - \nabla_\theta \E_{S} L(\theta; S)$ but that would disconnect this from practice. So to avoid that may be we can manipulate it the foll. way?}. Since $S \perp Q |C$:
\begin{align}
   & \E_{C}\E_{(S,Q)|C} \brck{\paren{\bI - \alpha \nabla_\theta^2 L(\theta; S)} \nabla_{\phi} L(\phi(\theta, S); Q)} \\
   & =\E_{C}\E_{(S,Q)|C} \brck{\paren{\bI - \alpha \nabla_\theta^2 L(\theta; S)} \paren{\nabla_{\phi} L(\phi(\theta, S); Q) - \nabla_{\phi} L(\phi(\theta); Q) + \nabla_{\phi} L(\phi(\theta); Q)}} \\
   &= \E_{C}\brck{\paren{\bI - \alpha \nabla_\theta^2 R_C(\theta)}   \nabla_{\phi} R_C(\phi(\theta))}\\
    & \qquad + \E_{C}\E_{(S,C)|Q}\brck{\paren{\bI - \alpha {\nabla_\theta^2 L(\theta; S)}} \paren{\nabla_{\phi} {L(\phi(\theta, S); Q)} - \nabla_{\phi} {L(\phi(\theta); Q)}}}
%   &= \E_{C}\brck{\paren{\bI - \alpha {\nabla_\theta^2 R_C(\theta)}}  \E_{(S,Q)|C}  \brck{\nabla_{\phi} {L(\phi; Q)}}}
\end{align}

Here $R_C(\theta)$ is the true risk of the task with $C$ classes. Note that the above simplification is not so straight forward for last-layer methods. For a $\mu$ smooth loss $L$, the second term in the expected meta-gradient:
\begin{align}
    \norm{\nabla_{\phi} {L(\phi(\theta, S); Q)} - \nabla_{\phi} {L(\phi(\theta); Q)}} &\leq \mu \|\phi(\theta, S) - \phi(\theta)\| \\
    & = \mu \alpha \|\nabla L(\theta; S) - \E_S \nabla L(\theta; S)\|
\end{align}

\am{Not sure about this but may be if we assume bounded variance of gradients on each task, then we can argue for $\sup_{S}  \|\nabla L(\theta; S) - \E_S \nabla L(\theta; S)\|$ to be bounded. But that may be loose. So instead we may have to bound the latter directly by a small value (which is stronger than assuming bounded variance)}

In the first order approx. of MAML, we drop $\paren{\bI - \alpha {\nabla_\theta^2 R_C(\theta)}}$ from the expected-meta gradient (on a particular task). In the case of \fixml the meta-gradient would be: \os{Here $\E_{Q | C}$ is used but $\phi$ also depends on $S$}\am{But in this case we are fixing the support right?}.

\begin{align}
   & \E_{C}\brck{\paren{\bI - \alpha {\nabla_\theta^2 L(\theta; S)}}  \E_{Q|C} \nabla_{\phi} {L(\phi; Q)}}
\end{align}

The first-order approximation of this meta-gradient would involve dropping the term $\paren{\bI - \alpha {\nabla_\theta^2 L(\theta; S)}}$ which may indeed be a bad approximation. One reason can be that the true risk of a task (loss evaluated over all possible supports) may be smoother than the loss function on a single support. In other words:

\begin{align}
        \norm{\nabla_\theta^2 \E_S L(\theta; S)}  < \norm{\nabla_\theta^2 L(\theta; S)}  \qquad \textrm{or,} \qquad
    \norm{\nabla_\theta^2 R_C(\theta)} <  \norm{\nabla_\theta^2 L(\theta; S)}
\end{align}

This may indicate that it is probably OK to drop second order term for \ml and not incur too much bias, but same can't be said for \fixml. The first-order approx. (biased gradient) for \fixml may be bad given that \fixml is itself a biased version of the \ml objective.

% \clearpage

% \paragraph{Implementation} The test set evaluation for all methods was done by sampling $2000$ random tasks with different $(S,Q)$ pairs from the test (novel) classes of the respective datasets. We empirically observe, that training with higher number of tasks (4-8) in a task mini-batch is particularly useful when training with lower number of $5$ ways since the higher batch size speeds up the convergence. On the other hand, for higher ways (like 20-way) this may deteriorate performance owing to overfitting on the train task distribution. Additionally, for \fixml we also find it helpful to train with a varying number of query points per class in a single task. 

% \clearpage

\begin{figure*}[ht]
    \begin{minipage}[b]{0.32\textwidth}
    \centering
    \includegraphics[width=\linewidth]{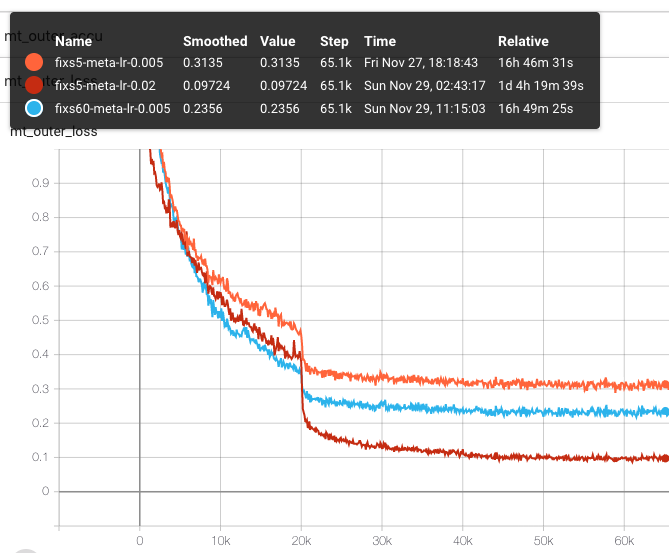}
    \captionsetup{labelformat=empty}
    % \caption*{(train)}
    \end{minipage}\hfill
    \begin{minipage}[b]{0.32\textwidth}
    \centering
    \includegraphics[width=\linewidth]{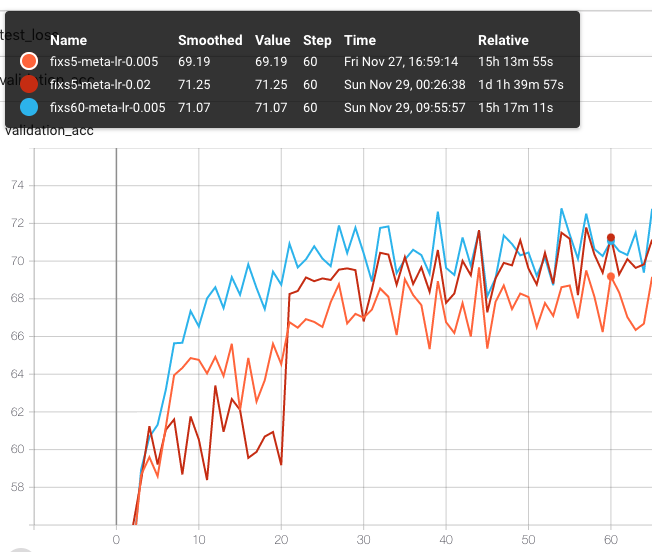}
    \captionsetup{labelformat=empty}
    % \caption*{(val)}
    \end{minipage}\hfill
    \begin{minipage}[b]{0.32\textwidth}
    \centering
    \includegraphics[width=\linewidth]{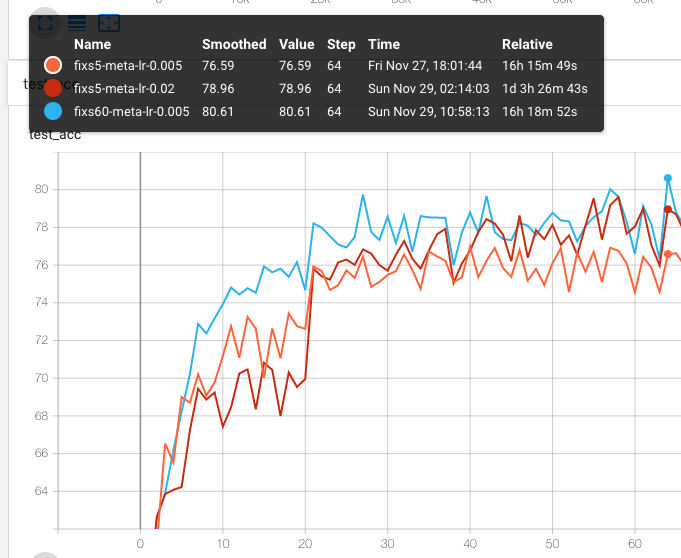}
    \captionsetup{labelformat=empty}
    % \caption*{(test)}
    \end{minipage}\hfill
    \begin{minipage}[b]{0.32\textwidth}
    \centering
    \includegraphics[width=\linewidth]{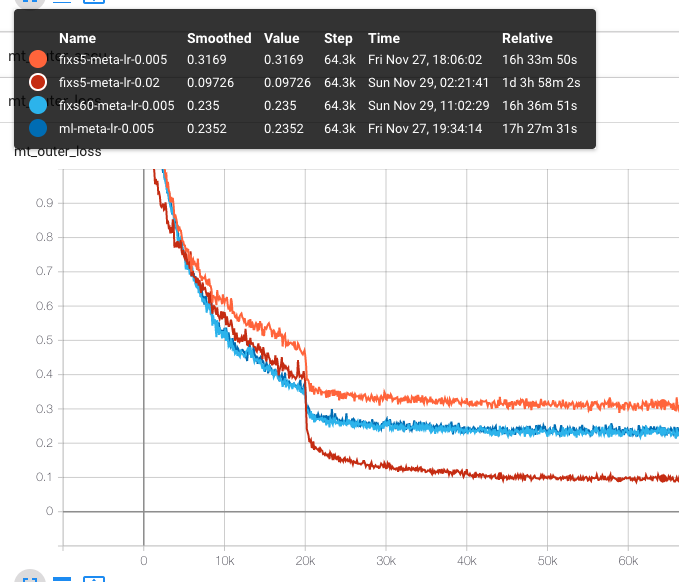}
    \captionsetup{labelformat=empty}
    % \caption*{(train)}
    \end{minipage}\hfill
    \begin{minipage}[b]{0.32\textwidth}
    \centering
    \includegraphics[width=\linewidth]{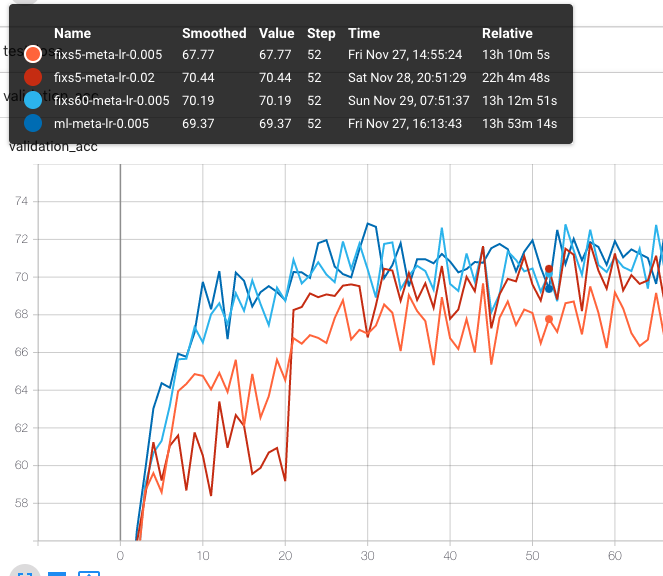}
    \captionsetup{labelformat=empty}
    % \caption*{(val)}
    \end{minipage}\hfill
    \begin{minipage}[b]{0.32\textwidth}
    \centering
    \includegraphics[width=\linewidth]{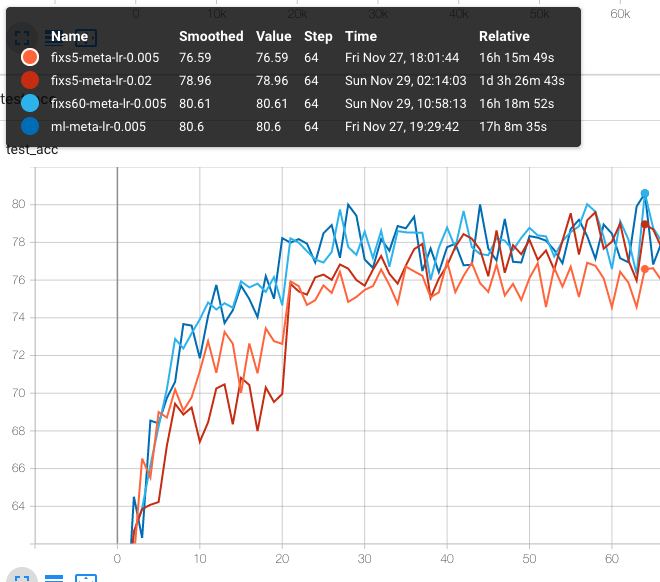}
    \captionsetup{labelformat=empty}
    % \caption*{(test)}
    \end{minipage}
    % \begin{minipage}[b]{0.32\textwidth}
    % \centering
    % \includegraphics[width=\linewidth]{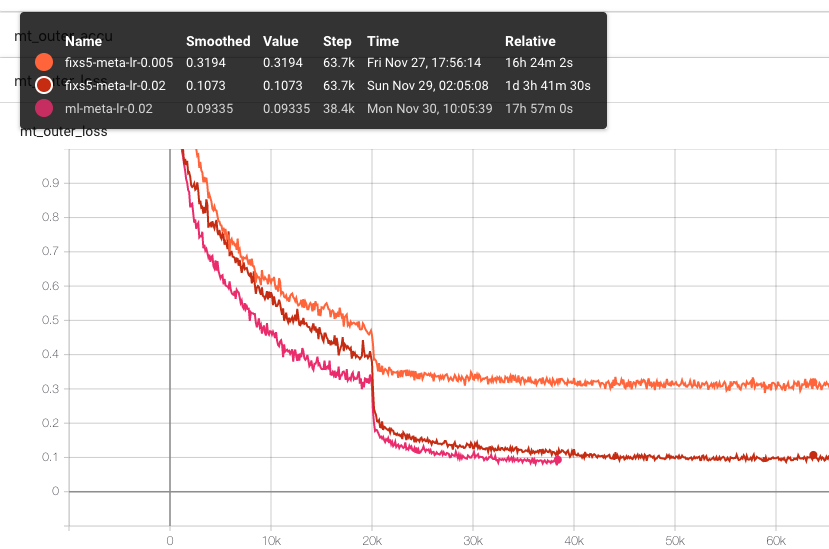}
    % \captionsetup{labelformat=empty}
    % \caption*{(train)}
    % \end{minipage}\hfill
    % \begin{minipage}[b]{0.32\textwidth}
    % \centering
    % \includegraphics[width=\linewidth]{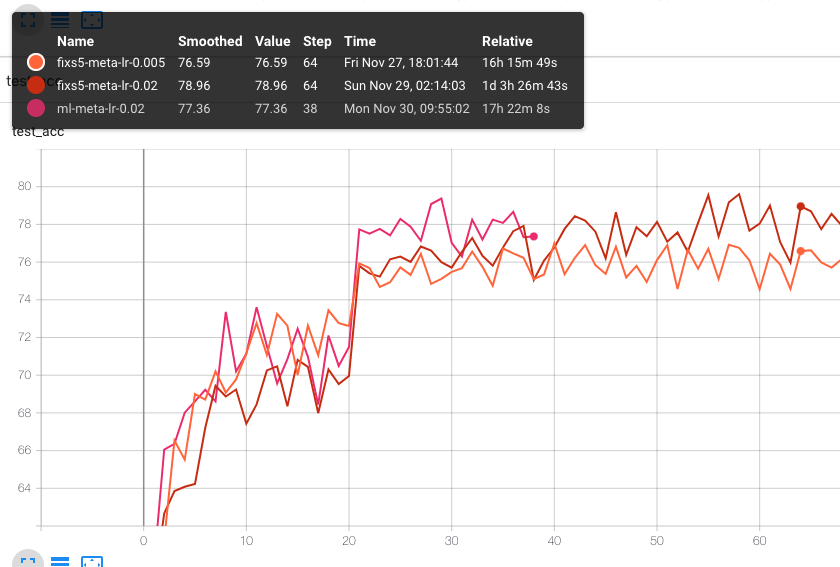}
    % \captionsetup{labelformat=empty}
    % \caption*{(test)}
    % \end{minipage}
    % \caption{$\alpha=0.5$}
    \label{fig:init-methods}
\end{figure*}

\begin{figure*}[ht]
    \begin{minipage}[b]{0.32\textwidth}
    \centering
    \includegraphics[width=\linewidth]{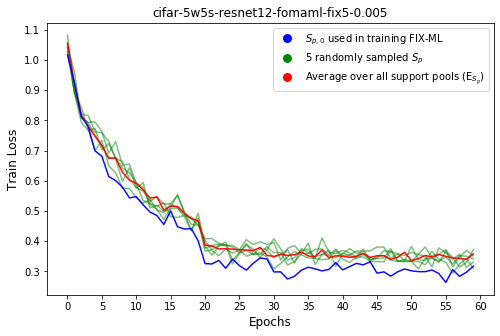}
    \captionsetup{labelformat=empty}
    % \caption*{(train)}
    \end{minipage}\hfill
    \begin{minipage}[b]{0.32\textwidth}
    \centering
    \includegraphics[width=\linewidth]{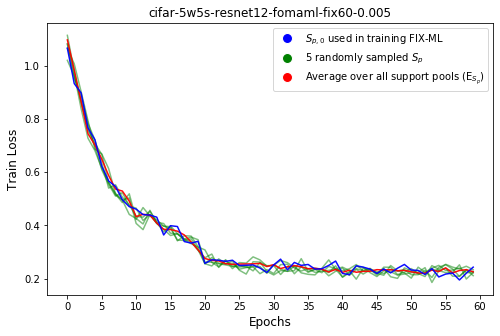}
    \captionsetup{labelformat=empty}
    % \caption*{(val)}
    \end{minipage}\hfill
    \begin{minipage}[b]{0.32\textwidth}
    \centering
    \includegraphics[width=\linewidth]{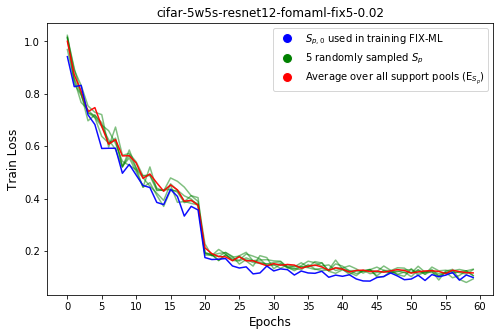}
    \captionsetup{labelformat=empty}
    % \caption*{(test)}
    \end{minipage}\hfill
    % \caption{$\alpha=0.5$}
    \label{fig:init-methods=trajectory}
\end{figure*}

\begin{figure}
    \centering
    \includegraphics[width=0.5\linewidth]{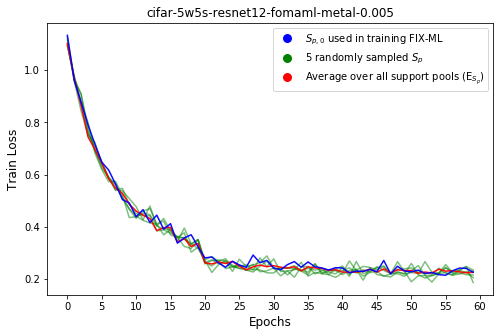}
    \caption{Losses along the optimization trajectory for meta-learning}
    \label{fig:my_label}
\end{figure}

\clearpage
